# Supplementary material for: Learning to Navigate Intersections with Unsupervised Driver Trait Inference
Source: arXiv:2109.06783 source file (2022-03-01)
Supplement: Supplementary file 1 [file Appendix.tex]

\section{Appendix}
\label{sec:append}
Not provided in the submitted version
